# Supplementary material for: Optimization-Based Quadrupedal Hybrid Wheeled-Legged Locomotion
Source: arXiv:2107.07507 source file (2021-07-15)
Supplement: Supplementary file 1 [file appendix.tex]

\section{Appendix} \label{sec:appedix}
Here we provide the mapping required between the Euler angles $\boldsymbol{\theta}=\begin{bmatrix} \theta_x & \theta_y & \theta_z \end{bmatrix}^{\top}$ and $\boldsymbol{\omega}$. This can be done by recalling that the order of application of the Euler angles is yaw-pitch-roll, as mentioned in Section \ref{sec:motion_planning_hybrid}:
\\
\begin{equation}
    \boldsymbol{\omega}=\begin{bmatrix} cos(\theta_y)cos(\theta_z) & -sin(\theta_z) & 0 \\  cos(\theta_y)sin(\theta_z) & cos(\theta_z) & 0 \\ -sin(\theta_y) & 0 & 1\end{bmatrix}\begin{bmatrix} \dot{\theta}_x \\ \dot{\theta}_y \\ \dot{\theta}_z \end{bmatrix}=\boldsymbol{C}(\boldsymbol{\theta})\dot{\boldsymbol{\theta}}
\end{equation}
By deriving this equation, the expression if $\ddot{\boldsymbol{\theta}}$ can be found:
\begin{subequations} \label{math: mapping}
\begin{alignat}{4}
    & \boldsymbol{\dot{\omega}}=\boldsymbol{\dot{C}}(\boldsymbol{\theta}, \boldsymbol{\dot{\theta}})\boldsymbol{\dot{\theta}}+\boldsymbol{C}(\boldsymbol{\theta})\boldsymbol{\ddot{\theta}} \\
    & \boldsymbol{\ddot{\theta}}=\boldsymbol{C}(\boldsymbol{\theta})^{-1}(\boldsymbol{\dot{\omega}}-\boldsymbol{\dot{C}}(\boldsymbol{\theta}, \boldsymbol{\dot{\theta}})\boldsymbol{\dot{\theta}})
\end{alignat}
\end{subequations}
The determinant of $\boldsymbol{C}(\boldsymbol{\theta})$ is $cos(\phi)$, therefore the matrix is singular when $\phi=k\frac{\pi}{2}, \ k=1,3,5,...$, but those values of $\phi$ would represent a very unlikely orientation of the base, therefore the mapping matrix is assumed to be always safely invertible.
\\
To recap, the procedure for finding the value for $\boldsymbol{\ddot{\theta}}$ according to the notation introduced previously) is schematized in the following pipeline:
\[ \boldsymbol{\theta}, \ \boldsymbol{\dot{\theta}} \quad \overset{\boldsymbol{C}(\boldsymbol{\theta})}{\longrightarrow} \quad \boldsymbol{\omega} \quad \overset{\text{eq. \ref{math: srbd2}}}{\longrightarrow} \quad \boldsymbol{\dot{\omega}} \quad \overset{\boldsymbol{\dot{C}}(\boldsymbol{\theta}, \boldsymbol{\dot{\theta}})}{\longrightarrow} \quad \boldsymbol{\ddot{\theta}}\]
